# Supplementary material for: Granular superconductivity and magnetic-field-driven recovery of macroscopic coherence in a cuprate/manganite multilayer
Source: arXiv:1512.03263 ancillary file (2016-11-13)
Supplement: Supplementary file 1 [file supplemental_material.pdf]

*Supplemental Material for*

# Granular superconductivity and magnetic-field-driven recovery of macroscopic coherence in a cuprate/manganite multilayer

B.P.P. Mallett[1#], J. Khmaladze[1#], P. Marsik[1#], E. Perret[1], A. Cerreta[1], M. Orlita[2], N. Biškup[3], M. Varela[3], C. Bernhard[1*]

1. University of Fribourg, Department of Physics and Fribourg Center for Nanomaterials, Chemin du Musée 3, CH-1700 Fribourg, Switzerland

2. Laboratoire National des Champs Magnétiques Intenses, CNRS-UJF-UPS-INSA, avenue des Martyrs, 38042 Grenoble, France

3. Departamento de Fısica Aplicada III, Instituto Pluridisciplinar, Universidad Complutense de Madrid, Spain

*correspondence to: christian.bernhard@unifr.ch

**The Supplemental Material includes:**

Sample growth and characterization
Magneto-transport measurements
Magnetization measurements
Ellipsometry measurements
Analysis of THz ellipsometry data
Transmission experiments
Effective-medium model

References

Figures S1 to S8

## Sample growth and characterisation

Thin films of $Pr_{0.5}La_{0.2}Ca_{0.3}MnO_3$ (PLCMO), $YBa_2Cu_3O_{7-\delta}$ (YBCO), and PLCMO (20nm)/YBCO (7,9 and 20nm)/PLCMO (20nm) trilayers were grown on $La_{0.3}Sr_{0.7}Al_{0.65}Ta_{0.35}O_3$ (LSAT) substrates by pulsed laser deposition (PLD). The general growth procedure for such films is described in detail in Ref. [1]. For these specific films, we have used a lower laser fluence of 1.4 $J/cm^2$ and an oxygen partial pressure of 0.36 mbar. Figure S1 shows representative reflection high energy electron diffraction (RHEED) patterns for our films. They reveal diffraction spots up to the $2^{nd}$ order, (02), indicating well-ordered, flat surfaces.

All trilayer samples were *ex-situ* post-growth annealed in oxygen at 700ºC for 4 hours, then 600 ºC for 14 hours before cooling to room temperature (in oxygen) at approximately 3ºC per minute. All characterization measurements (other than RHEED), were made after this *ex-situ* annealing process.

The PLCMO/YBCO bilayers were grown on LSAT substrates and to protect the very thin YBCO layer from degradation due to interaction with the ambient, we have added a 1 nm thick $LaAlO_3$ capping layer on top. The bilayer samples were *in-situ* annealed in oxygen only.

X-ray reflection and diffraction of our films was measured using a 4-cycle diffractometer (RIGAKU Smartlab). Typical x-ray diffraction data are shown in Fig. S2**A** and confirm that our films are of good epitaxial quality and without observable spurious phases. The inset to Fig. S2**A** highlights the Kiessig fringes of the PLCMO (004) reflection. Typical x-ray reflection data for our films are shown in Fig. S2**B** and are modelled and fitted using the software *GenX* developed by M. Björck and A. Viklund. The x-ray reflection data confirm the YBCO and PLCMO film thicknesses expected from the growth conditions and yield a typical average surface roughness of the films of about 1nm for YBCO and 0.5nm for PLCMO (corresponding to about 1 unit-cell 'roughness' for each material).

We have also studied a PLCMO (20 nm)/YBCO (7 nm)/PLCMO (20 nm) trilayer with cross-sectional scanning transmission electron microscopy (STEM) and electron energy-loss spectroscopy (EELS). STEM observations were carried out in a JEOL JEM-ARM200cF operated at 200 kV equipped with a spherical aberration corrector and a Gatan Quantum electron energy-loss spectrometer. Random noise was removed from the EELS data by using principal component analysis [2]. Chemical maps were produced by subtracting the background via a power law fit and integrating the remaining signal within 15-20 eV wide windows. Specimens were prepared in cross section by conventional methods: grinding and Ar ion milling.

Low magnification STEM images, shown in Fig. S3, reveal that the layers are flat and continuous over lateral distances of the order of a few microns. No secondary phases or pinholes were detected. Atomic resolution images exhibit flat, coherent interfaces confirming epitaxial growth. Some step disorder can be observed in the form of occasional interface steps one unit-cell high. These occasional steps result in antiphase boundaries within the YBCO layer. Regarding this layer, the main type of defect that is found in the YBCO is a relatively low density of stacking faults in the form of double planes of CuO chains (giving rise to a darker contrast, such as those darker stripes observed in the lower panels of **A**). Neither these defects, which resemble a Y-124-like structure and are relatively common in YBCO, nor the interface steps compromise the

integrity or crystallinity of the YBCO layers. These images have been obtained with a high-angle annular dark field (HAADF) detector in so-called *Z*-contrast mode for which the scattering cross section is roughly proportional to the square of the atomic number *Z*. The heavier elements, such as La, Pr, Y, and Ba thus appear brighter, whereas the lighter elements, such as Mn and Cu appear darker. The O atoms are not visible.

The middle panels in Fig. S3**B** show, in false color, chemical maps across the interface as acquired by EELS (note that the Cu L2,3 and Pr M4,5 absorption edges overlap and so these ions cannot be individually resolved). The right panel shows the integrated intensities along the growth direction (i.e. along the *c*-axis direction). These data sets reveal that the PLCMO/YBCO interfaces are chemically sharp with minimal ion inter-diffusion across the interface.

**Magneto-transport measurements**

Temperature and magnetic-field dependent resistance measurements were made in a Quantum Design PPMS whilst using a Keithley 2602 digital multi-meter to measure the voltage from a set current. Current and voltage lead contacts were made either on top of the film (i.e. to the PLCMO layer, as for Figs. 1a-d) and Fig. 3) or directly onto the edge of the film/substrate (for Figs. 1e) and f)) as shown schematically, along with approximate dimensions, in Fig. S4a.

Figure S4b shows *R*-*T* curves at 9 Tesla for field directions parallel and perpendicular to the film surface (perpendicular and parallel to the *c*-axis respectively) and in zero-field. This PLCMO/YBCO/PLCMO sample has a slightly lower $T_c$ than the one discussed in the paper. As can be readily seen from the data, for both field orientations the large magnetic field restores the coherence of the SC state. Note that the broader transition in the perpendicular field orientation is expected from the high vortex density in the $CuO_2$ layers of the YBCO. Indeed, Fig. S4c shows that the voltage above the critical current density exhibits a sharp minimum when the magnetic field is parallel to the $CuO_2$ planes, just as expected for a strongly anisotropic superconductor like YBCO.

As is evident from Figs. 1 and 3 in the manuscript, there are significant dependencies of the electrical transport response of our multilayers on the magnitude and history of the temperature, magnetic field and applied current. Therefore, we detail below the measurement conditions for the data shown in the manuscript.

*Figs. 1a, b and c)*: The data were taken whilst cooling in a magnetic field, applied parallel to the film, as specified in the legends. The applied current was 10 µA (although, in fact, above a resistance value of the sample of about 0.2 MΩ this current was automatically reduced by our measurement electronics so as not to exceed the internal voltage limit). After each measurement the sample was heated to 300 K in zero-field before subsequent measurements.

*Fig. 1d):* These measurements were performed after zero-field and zero-current cooling from 300K for each temperature shown. At the specified temperature, the magnetic field was applied parallel to the film and swept from 0T to 9T, then to -9T and finally back to 9T. The applied current was 200 nA. The difference in the measurement procedure for Fig. 1a) and Fig. 1d) leads to, for example, the difference in the *R*-values at 40 K and 9 Tesla. The difference in *R*-values at zero field and 100 to 150 K are due to the

combined effects of the current history and a small offset voltage which most likely originates from charging effects in the top PLCMO layer and also exhibits hysteresis effects and furthermore has a much stronger effect on $R$ at 200 nA than at 10 μA.

*Figs. 1e and f):* The sample was cooled to the specified temperature in the indicated magnetic field and an applied current of 10 μA.

*Figs 3a and b):* These data were taken whilst cooling in a magnetic field, applied parallel to the film, as specified in the legend. The applied current is specified in the legends also. After each measurement the sample was brought to 300 K in zero-field before subsequent measurements.

**Magnetization measurements**

Magnetization measurements were made using a PPMS vibrating sample magnetometry system. The contribution from the LSAT substrate is well described by a temperature-independent diamagnetic term plus a paramagnetic term that were determined from measurements of the substrate before deposition of the film. In Fig. 4c of the paper this substrate contribution has been subtracted.

Figure S5a) shows a magnetization loop at 10 K for the PLCMO (20 nm)/YBCO (7 nm)/PLCMO (20 nm) trilayer with the magnetic field parallel to the film surface. The inset shows that the size of the coercive field is about 50 mT.

Figure S5b) and c) shows the magnetic response of the trilayer in a small fields applied perpendicular to the film surface (i.e. perpendicular to the $CuO_2$ layers of the YBCO). The magnetization has been measured with the VSM of the PPMS for both zero-field-cooling (ZFC) and field-cooling (FC) modes. The data reveal large differences between the ZFC and FC data and a strong variation in the low-temperature part of the ZFC data with the applied field. The FC curves are governed by the ferromagnetic signal of the PLCMO layers and show hardly any sign of a SC response, except for a weak anomaly below 20 K. In contrast, the ZFC data undergo large changes below about 45 K that can be associated with the granular SC state of the YBCO layer. Notably, this low-temperature signal varies a lot from strongly diamagnetic at 2 mT, to weakly diamagnetic at 5 mT, back to strongly diamagnetic at 10 mT and even becomes paramagnetic at 20 mT.

Such an anomalous behavior is not untypical for a thin film with a spatially inhomogeneous SC response. It is governed by the large demagnetization effects that occur when the field is perpendicular to the film plane. The demagnetization factor is strongly dependent on the spatial distribution of the magnetic flux density within the sample. A local variation in the flux density, which hardly affects the average magnetization of the sample, thus can give rise to a large change of the magnetic signal. The interpretation of these ZFC data in terms of an average magnetization density is therefore not straight-forward. It requires further information about the local distribution of the magnetization density of this granular SC state which is the subject of our ongoing research, for example with the magnetic force microscopy (MFM) technique.

Finally, note that the corresponding magnetization curves for the field parallel to the film plane show no sign of such a diamagnetic or paramagnetic signal at low temperature. This is expected since the demagnetization effects and the SC response are at their minimum for this field geometry for which the SC current has to flow in the direction perpendicular to the film plane (and the $CuO_2$ planes of the YBCO).

**Ellipsometry measurements**

The temperature and frequency dependent optical response has been determined using three spectroscopic ellipsometers which cover a broad range of 3 – 52000 $cm^{-1}$. In the terahertz regime (3-70 $cm^{-1}$) we used a home-build time-domain THz ellipsometer that is based on a femtosecond laser and photoconductive antennas in rotating analyzer configuration with wire-grid polarizers [3]. For the far-infrared (70-700 $cm^{-1}$) and mid-infrared (500-4500 $cm^{-1}$) ellipsometry we used a home-build setup attached to a Bruker 113v as described in Ref. [4]. In the far-infrared we used a rotating analyzer scheme with an additional Si-prism compensator at low frequencies of 70-165 $cm^{-1}$. In the mid-infrared range we utilized a ZnSe-prism based rotating compensator. Finally, the near-infrared to ultraviolet data at 4000-52000 $cm^{-1}$ (0.5-6.5 eV) were obtained with a Woollam VASE ellipsometer.

The raw ellipsometric data of the substrate/film samples in the form of the complex ratio $\rho$ of the p- and s- polarized Fresnel coefficients, $\rho=r_p/r_s=\tan\Psi\cdot\exp(i\Delta)$, are commonly expressed in terms of the ellipsometric angles $\Psi$ and $\Delta$. These have been recalculated to obtain the pseudo-dielectric function $\langle\varepsilon\rangle$ of the substrate/film system (see Fig. S6) using the expression $\langle\varepsilon\rangle = \sin^2\varphi\left[1+\tan^2\varphi\left(\frac{1-\rho}{1+\rho}\right)^2\right]$, where φ is the angle of incidence (φ=75° for the THz, FIR and MIR and φ=70° for the NIR/VIS/UV).

The effective response of the trilayer (as shown in Fig. 2) has been obtained by fitting with a standard optical transfer matrix model of the ambient/film/substrate system in a point-by-point manner. The dielectric function of the LSAT substrate, as measured with ellipsometry under the same conditions, has been used as input. The wave-like structures in Fig. 2 for temperatures above 70 K and starting at 13$cm^{-1}$ and decreasing in strength towards higher wavenumber are most likely experimental artefacts due to an interference effect from spurious reflections (e.g. backside reflections off the substrate) and the transformation from the measurement in the time-domain to the frequency-domain.

**Analysis of THz ellipsometry data**

In the THz range, due to the small sample size to wavelength ratio, diffraction effects influence the raw data of both the substrate and the trilayer/substrate samples. To remove these effects, we calculated the difference spectra $\Delta\langle\varepsilon(T)\rangle = \langle\varepsilon(T)\rangle - \langle\varepsilon(300K)\rangle$ and fitted them with a differential optical model. The input for the room-temperature response of the trialyer has been obtained from the extrapolation of a Drude-Lorentz model fit of the far-infrared data which yields nearly constant values of $\varepsilon_1 \approx 29$ and $\sigma_1 \approx 232\ \Omega^{-1}cm^{-1}$ in the THz range.

## Transmission measurements

The optical transmission measurements at 4.2 K in magnetic fields up to 11 T have been carried out at the Laboratoire National des Champs Magnétiques Intenses (LNCMI) in Grenoble using a Bruker 113v for the THz and a 66v Fourier-transform spectrometer for the MIR and NIR ranges. The signal from the film was referenced *in situ* against a bare LSAT substrate. In the intermediate range from 70-1000cm$^{-1}$ (8.5-124 meV) the transmission falls to zero due to absorption by optically-active phonons in the LSAT substrate.

The field-dependent relative transmission data in the mid-infrared range, presented in Fig. 4a of the manuscript, have been fitted using a Drude-Lorentz model, based on the zero-field data obtained from ellipsometry (as shown in Fig. 2a). One (at 4 T and 6 T) or two (at 8 T and 11 T) additional Lorentzian bands have been added to reproduce the pronounced transmission minimum around 3000-4000 cm$^{-1}$. The weight of the interband transition around 10,000 cm$^{-1}$ has also been allowed to vary, whereas all other parameters have been kept constant. The optical conductivity obtained with this model is shown in Fig 4b of the manuscript.

Fig. S7 shows the zero-field THz transmission data of the PLCMO/YBCO/PLCMO trilayer normalized to the one of a bare LSAT substrate (for 23μm and 75μm mylar beamsplitters that cover different spectral ranges). For comparison, we also show corresponding data of a single 20 nm thick YBCO film on LSAT. The spectral resolution of the experimental data has been set to 4 cm$^{-1}$ in order to remove the Fabry-Pérot fringes due to the double-side polished and 0.5 mm thick LSAT substrate. The trilayer data reveal a resonance below 30 cm$^{-1}$ that is the signature of the transverse plasma mode which has been detected with ellipsometry and is shown in Fig. 2 of the manuscript. This feature is absent for the single YBCO layer for which the transmission is well accounted for by the sum of a purely inductive term, due to the loss-free response of the superconducting condensate, and a Drude-term with a finite scattering rate. The parameters for the trilayer model are similar but not identical to the ones used to describe the ellipsometry data in Fig. 2 of the manuscript, this may be owed to the circumstance that different trilayer samples (grown on single- and double-side polished substrates, respectively) have been used for these experiments. This modeling also gives rise to spurious features above 40 cm$^{-1}$ which arise from the FFT low-pass filtering that was necessary to remove the Fabry-Pérot oscillations in order to compare the model with the low-resolution experimental data. Irrespective of these technical details, these transmission data underline that the low-energy mode, as seen from the THz ellipsometry data in Fig. 2, is a real feature that is not caused, for example by diffraction effects.

## Effective-medium model

The ellipsometric measurements have been performed at an incidence angle of 70° or 75°, but due to the refraction into the film and the substrate, the electric field inside the material probes mainly the in-plane dielectric response. The response of the trilayer thus can be considered as a linear combination of the contributions of the individual PLCMO and YBCO layers that are weighted according to their thicknesses. The temperature dependence of this combined response in the THz range is dominated by the YBCO layer

(since the PLCMO layers are insulating). To account for a granular structure of the YBCO layer, with superconducting domains and non-conducting boundaries that prohibit percolation, we treated the film as a mixed medium. For the modelling we used a simplified geometry in which the probing field is perpendicular to the blocking boundaries. This yields the Maxwell-Garnett-type effective medium dielectric function [5,6], $\varepsilon_{eff}$ , according to $\frac{1}{\varepsilon_{eff}} = f\frac{1}{\varepsilon_{SC}} + (1-f)\frac{1}{\varepsilon_{B}}$, where $\varepsilon_{SC}$ is the dielectric function of the superconducting domains with volume fraction *f*, and $\varepsilon_{B}$ is the dielectric function of the blocking boundaries.

The superconducting phase has been represented by a purely inductive term, $\varepsilon_{SC} = \varepsilon_{\infty} - \frac{\omega_{PL}^{2}}{\omega^{2}}$, with a plasma frequency $\omega_{PL}$ = 950 $cm^{-1}$. The latter value has been deduced from the spectral weight of the low-energy plasmonic mode (if one considers that this plasmonic mode originates only from the 7 nm thick YBCO layer one obtains the value of $\omega_{PL} \approx 2400$ $cm^{-1}$ that is quoted in the paper). A value of $\varepsilon_{\infty}$=30 has been used according to the measured effective dielectric constant at room temperature. For the boundaries we assumed a dielectric constant of $\varepsilon_{B}$=30+37i. The finite value of the imaginary part is required to account for the broadening of the low-energy plasma mode.

Figure S8 shows the obtained spectra for $\varepsilon_{1eff}$ and $\sigma_{1eff}$ as a function of the volume fraction, *f* , of the superconducting domains. It highlights that *f* needs to be rather close to unity in order to reproduce the very low resonance frequency of the plasma mode which in the experimental data is located at 7 $cm^{-1}$. Reasonably good agreement with the experimental data is obtained for *f*=0.996. Since $\varepsilon_{B}$ scales with (1-*f*), the *f*-value can reduced by increasing the real part of $\varepsilon_{B}$, i.e. for $\varepsilon_{B}$=300+370i the frequency of the plasmonic mode is reproduced at *f*=0.96. However, in the normal state data above 100K there is no evidence of such a large dielectric constant. The *f*-value also depends on the assumed geometry of the boundaries which can be expressed in terms of the so-called aspect ratio, q. For example, it gets reduced from *f*=0.996 for the above described planar geometry with q=1 (see Fig. S8) to *f*=0.992 for cylindric domains with q=1/2.

The agreement of the effective medium approximation with data has been further improved, as shown in Figs. 2b and c of the manuscript, by adding a Drude-term to the response function of the superconducting domains. This enhances the conductivity at frequencies above the plasmonic mode and it contributes to the broadening of the plasmonic mode. However, without the finite imaginary part of $\varepsilon_{B}$, the broadening from this Drude term is not sufficient to obtain a good description of the plasma mode.

One needs to keep in mind that this effective medium model provides a purely phenomenological description of the data. Nevertheless, the circumstance that a finite imaginary part of $\varepsilon_{B}$ is required to obtain a good description of the plasma mode seems inconsistent with the most simplistic picture of domain walls that are very thin and high insulating. On the other hand, it is not implausible that destructive interference effects, e.g. due to a phase mismatch of the superconducting order parameter, give rise to a dissipation that can be expressed in terms of a constant imaginary part of the dielectric function (within a limited frequency range).

## References


1. V.K. Malik *et al.*, Pulsed laser deposition growth of heteroexpitaxial $YBa_2Cu_3O_7/La_{0.67}Ca_{0.33}MnO_3$ superlattices on $NdGaO_3$ and $Sr_{0.7}La_{0.3}Al_{0.65}Ta_{0.35}O_3$ substrates, *Phys. Rev. B* **85**, 054514 (2012).

2. M. Bosman, M. Watanabe, D. T. Alexander, V. J. Keast, Mapping chemical and bonding information using multivariate analysis of electron energy-loss spectrum images, *Ultramicroscopy* **106**, 1024 (2006).

3. N. Matsumoto, T. Hosokura, T. Nagashima and M. Hangyo, Measurement of the dielectric constant of thin films by terahertz time-domain spectroscopic ellipsometry, *Opt. Letters* **36**, 265 (2011).

4. C. Bernhard, J. Humlicek, B. Keimer, Far-infrared ellipsometry using a synchrotron light source – the dielectric response of the cuprate high $T_c$ superconductors, *Thin Solid Films* **455**, 143 (2004).

5. J. C. Maxwell Garnett, Colours in metal glasses and in metallic films, *Phil. Trans. Royal Soc. London A* **203**, 385 (1904).

6. J. Humlicek, Infrared resonances of local fields and ellipsometric spectra of negative – refraction metamaterials, *Thin Solid Films* **519**, 2655 (2011).

**Fig. S1**

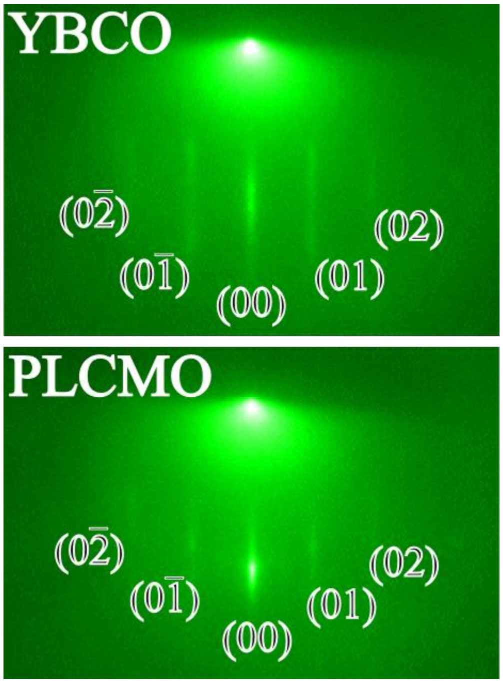


Fig. S1. Representative *in-situ* RHEED patterns for the YBCO layer and the (top-most) PLCMO layer. The ‘streaks’ are diffraction spots (0th to 2nd order) which indicate well-ordered, flat surfaces.

**Fig. S2**

A

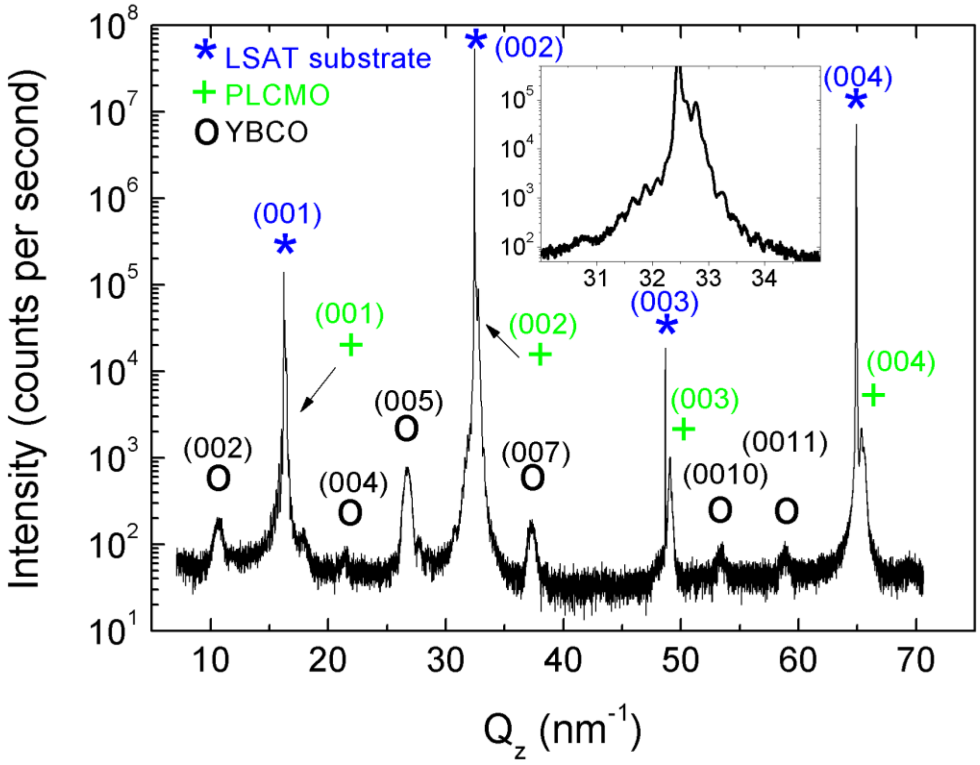


B

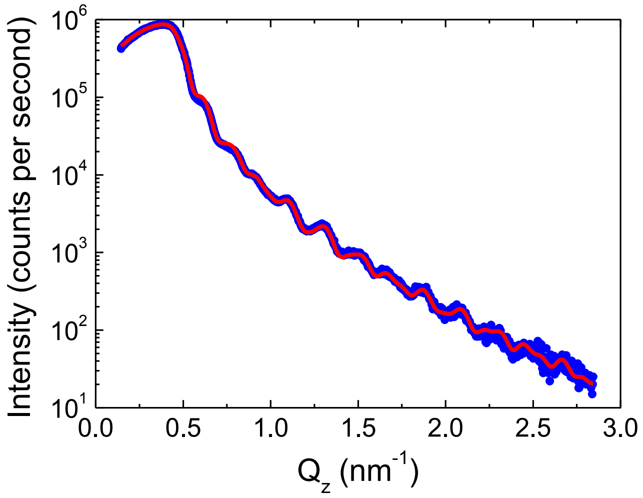


Fig. S2. **A,** A representative x-ray diffraction pattern with the (00l) reflections indicated for the pseudo-cubic unit-cells of LSAT and PLCMO. Qz is the reciprocal lattice vector length parallel to the c-axis of the film/substrate. **B**, Low-angle x-ray reflection data (blue points) and fit (red line) from which the thickness and roughness of the YBCO and PLCMO layers have been determined.

**Fig. S3**

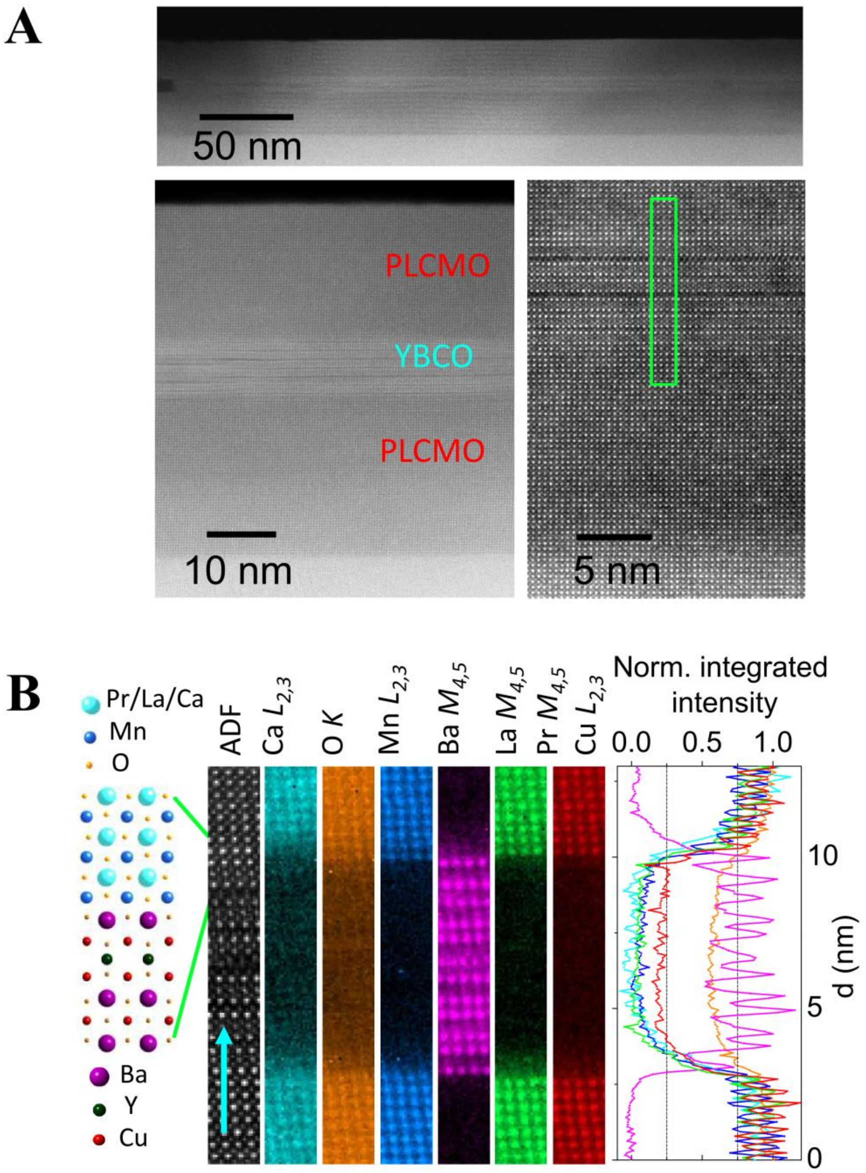


Fig. S3. STEM-EELS analysis of a PLCMO(20nm)- YBCO(7nm)- PLCMO(20nm) trilayer. **A,** High angle annular dark field (HAADF) images at low (top) and high (lower panels) magnifications. **B,** Chemical maps obtained from the area marked with a green rectangle in **A**. The different panels exhibit the simultaneously acquired ADF signal along with maps obtained from the Ca L2,3 (cyan) O K (orange), Mn L2,3 (blue), Ba M4,5 (magenta), La M4,5 (green)and Pr M4,5/Cu L2,3 (red) absorption edges, nominally around 346 eV, 528 eV,  640 eV, 781 eV, 832 eV, and 931 eV, respectively, (please, note that the Pr and Cu edges overlap). The sketch shows the interface structure. The panel at the right end exhibits the normalized integrated intensities for all chemical maps along the growth direction on a matching color code, averaged in the direction parallel to the interface. The blue arrow indicates the growth direction.

**Fig. S4**

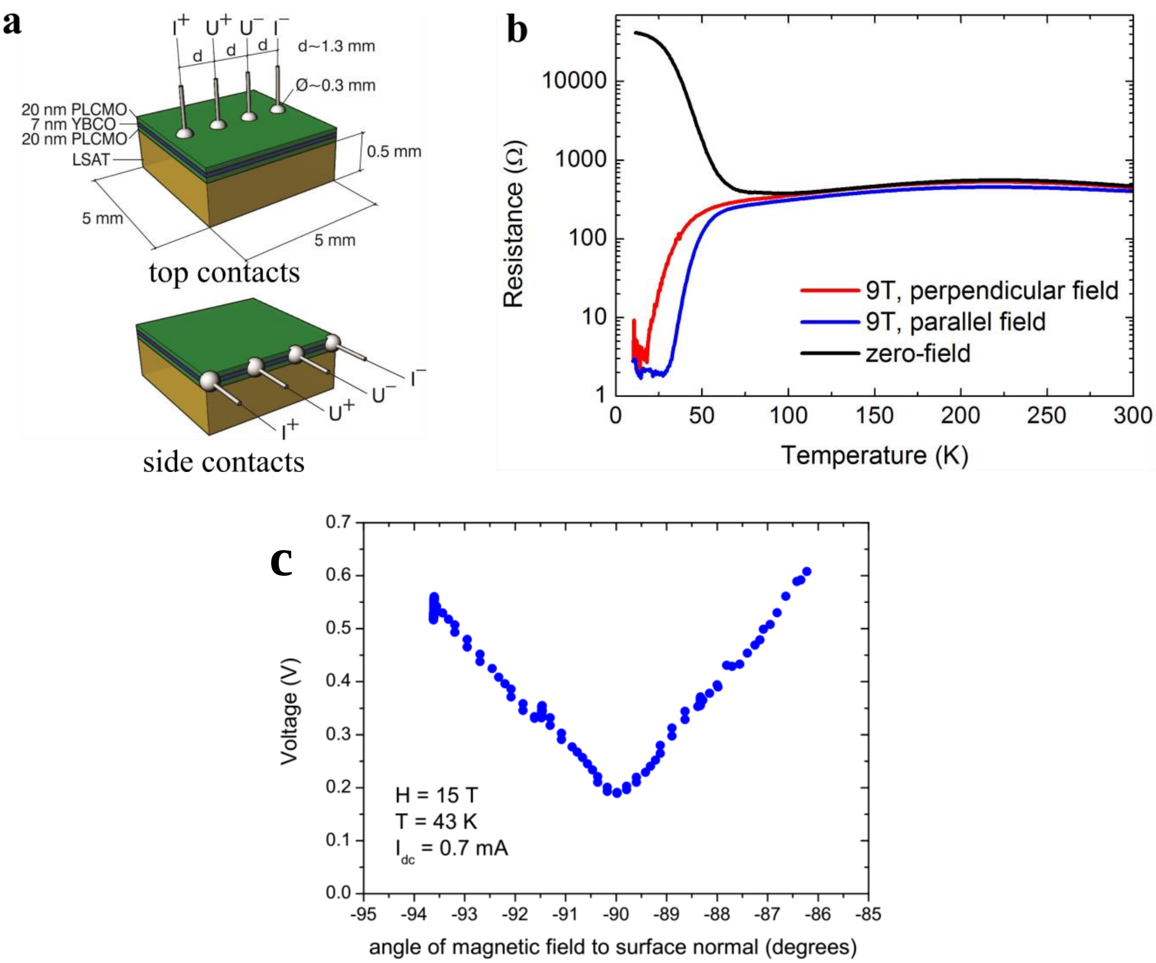


Fig. S4. **a,** Schematic diagrams of the measurement geometry for top and side contacts. Unless explicitly mentioned, the resistance measurements presented in this work were made using the top contact geometry. **b**, A comparison of *R*-*T* measurements on a PLCMO(20 nm)/YBCO(7 nm)/PLCMO(20 nm) trilayer in a 9T magnetic field orientated parallel and perpendicular to the film surface and in zero-field. **c**, Dependence of the voltage drop across a PLCMO(20 nm)/YBCO(7 nm)/PLCMO(20 nm) trilayer sample (in a 4-terminal measurement configuration) for a fixed current of 0.7 mA as the angle between the applied magnetic field and the normal of the film is altered. The current applied is slightly higher than $I_c$, the critical current of the superconductor (under these specific conditions). At -90 degrees the field is parallel to the film surface i.e. perpendicular to the c-axis of the YBCO.

**Fig. S5**

a)

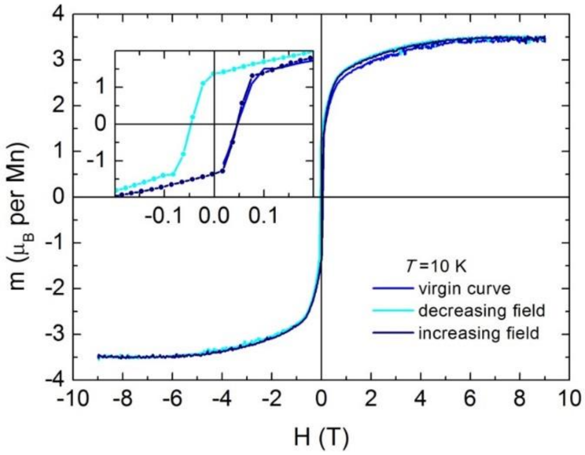


b)

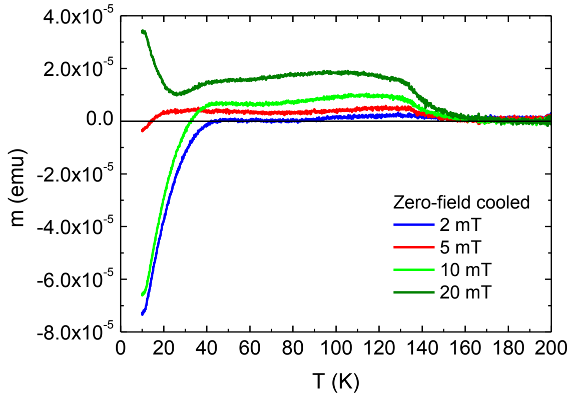


c)

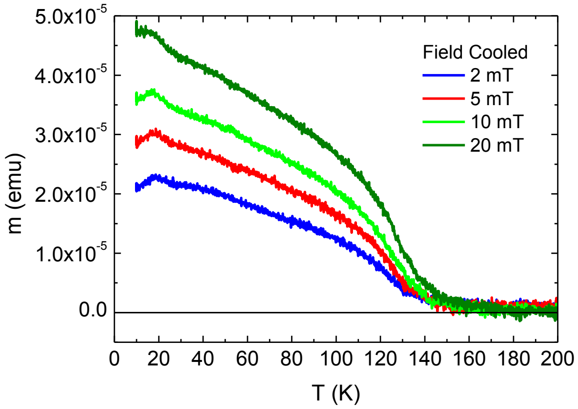


Fig. S5. a) Magnetization vs field of the PLCMO (20 nm)/YBCO (7 nm)/PLCMO (20 nm) trilayer at 10 K with the field parallel to the film surface. The inset highlights the data at low fields. b) Zero-field and c) field cooled magnetization of the trilayer for fields of 2, 5, 10 and 20 mT applied perpendicularly to the film surface (i.e. perpendicular to the $CuO_2$ layers of the YBCO).

**Fig. S6**

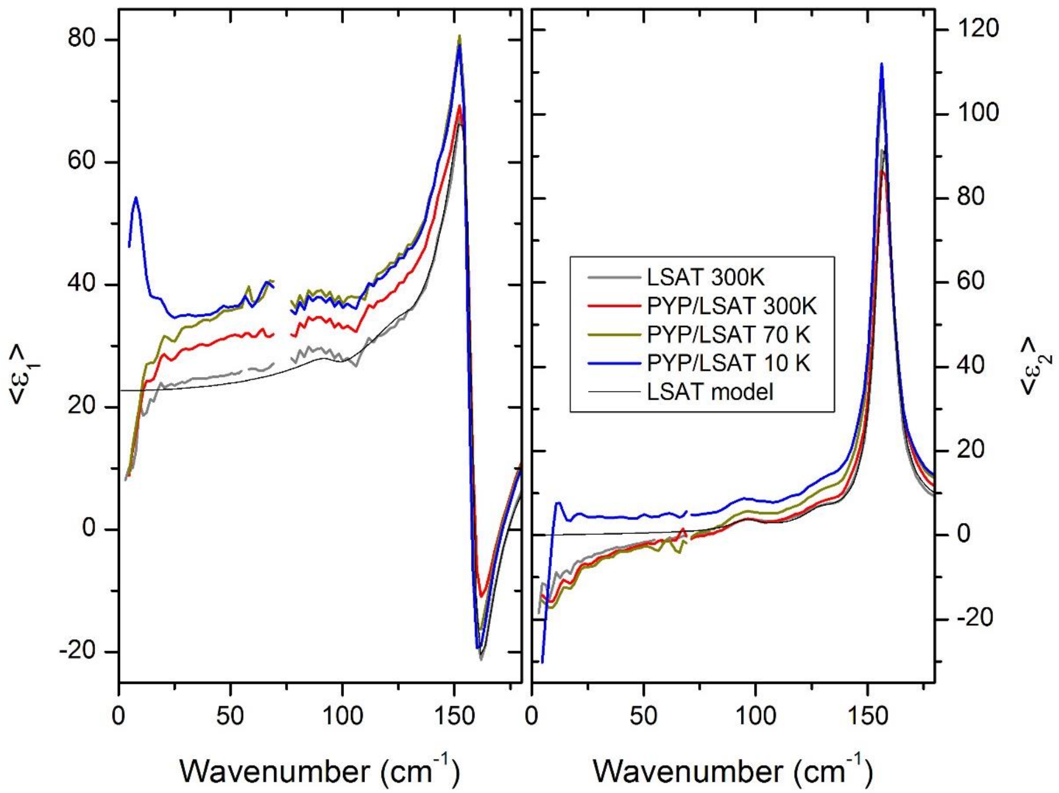


Fig. S6. Real and imaginary parts of the pseudo-dielectric functions of the PLCMO/YBCO/PLCMO/LSAT sample, the LSAT substrate, and the model for LSAT extrapolated from the far-infrared data The sharp feature at 157 $cm^{-1}$ is due to a phonon mode of the LSAT substrate. The changes of $<\varepsilon_1>$ with respect to the substrate are proportional to the real part of the optical conductivity of the film, $\sigma_{1film}$, while the changes in $<\varepsilon_2>$ are proportional to $\sigma_{2film}=-\varepsilon_0\omega\varepsilon_{1film}$.

**Fig. S7**

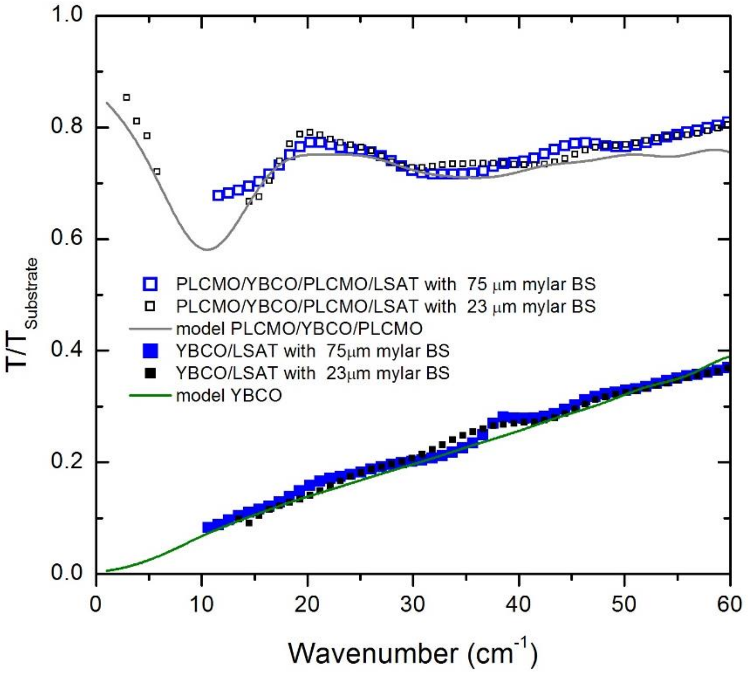


Fig. S7. THz transmission data, normalized with respect to the LSAT substrate, of the PLCMO/YBCO/PLCMO trilayer compared to a 20 nm thick YBCO film.

**Fig. S8**

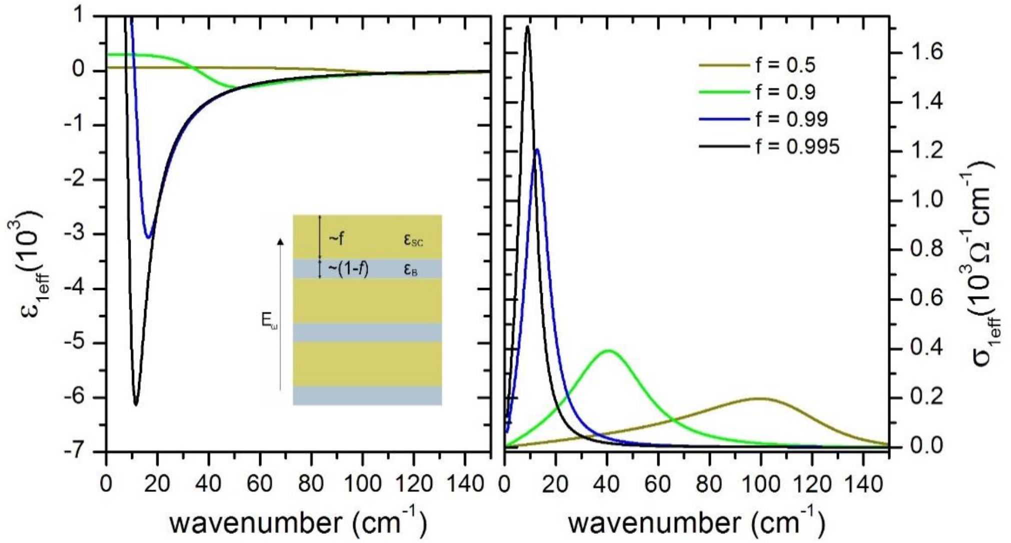


Fig. S8. Effective medium approximation for the THz response of a planar array of superconducting domains that are separated by dielectric layers that are perpendicular to the electric field vector (a sketch is shown in the inset). It shows the evolution of the plasmonic mode as a function of the volume fraction, *f*, of the superconducting material for the choice of parameters that is described in the paragraph "effective medium model".
